# Supplementary material for: Automatic Detection of Aedes aegypti Breeding Grounds Based on Deep Networks with Spatio-Temporal Consistency
Source: arXiv:2007.14863 source file (2021-11-27)
Supplement: Supplementary file 1 [file Appendix.tex]

\appendix
Aqui vão informações mais apropriadas para um apêndice.
